# Supplementary material for: Effects of inertia on conformation and dynamics of tangentially-driven active filaments
Source: arXiv:2209.07880 source file (2023-03-09)
Supplement: Supplementary file 1 [file supplementary.pdf]

# Effect of inertia on conformation and dynamics of active polymers

## Supplementary Material

### I. TANGENTIALLY DRIVEN ACTIVE POLYMER SIMULATIONS

#### A. Model definition

We use a tangentially-driven active polymer model identical to the model put forward by Isele-Holder et al. [1] to examine the effect of inertia on the conformational dynamics of active flexible filaments. The active filament is modelled as a flexible linear polymer composed of a sequence of  $N$  bead-like units connected via harmonic springs. The chains are under the influence of an active force which is tangential to the polymer backbone. Hence, the active force is directly coupled to the polymer conformation. The dynamics of each bead of an active polymer with mass  $m$  is described by the Langevin equation of motion:

$$m\ddot{\mathbf{r}}_i = -\gamma\dot{\mathbf{r}}_i - \sum_j \nabla_{\mathbf{r}_i} U(r_{ij}) + \mathbf{f}_i^a + \mathbf{f}_i^r, \quad (1)$$

in which  $\mathbf{r}_i$  is the coordinate of the bead  $i$  with the dots denoting derivatives with respect to time and  $\gamma$  is the effective friction coefficient of the bead.  $r_{ij} = |\mathbf{r}_j - \mathbf{r}_i|$  denotes the distance between bead  $i$  and  $j$  and  $U(r_{ij})$  is the potential energy of inter-particle interactions.  $\mathbf{f}_i^a$  and  $\mathbf{f}_i^r$  are the active and random thermal forces acting on the bead  $i$ , respectively.

The total potential energy of a bead  $U = U_{\text{Bond}} + U_{\text{excl}}$  includes contributions from springs connecting the monomer to its adjacent monomers along the chain backbone  $U_{\text{Bond}}$  and excluded volume potential  $U_{\text{excl}}$  between any two monomers which guarantees the self avoidance of the polymers. The bond potential used throughout our simulations is a harmonic oscillator potential:

$$U_{\text{Harmonic}}(r) = (1/2)k_s(r - \ell)^2, \quad (2)$$

in which  $\ell$  is the length of the spring at rest and  $k_s$  is its stiffness. The excluded volume interactions between any two beads, bonded or non-bonded, at a distance  $r$  are modelled by the truncated and shifted Lennard-Jones potential, *i.e.*, Weeks-Chandler-Andersen (WCA) potential,

$$U_{\text{excl}}(r) = 4\epsilon \left[ \left( \frac{\sigma}{r} \right)^{12} - \left( \frac{\sigma}{r} \right)^6 + \frac{1}{4} \right], \quad r < r_{\text{cut}} \quad (3)$$

where  $\epsilon$  sets the strength of pairwise interaction energy, and  $r_{\text{cut}} = 2^{1/6}\sigma$  is the cutoff distance such that  $U_{\text{excl}}(r > r_{\text{cut}}) = 0$ .

By defining the bond vector  $\mathbf{r}_{i,i+1} = \mathbf{r}_{i+1} - \mathbf{r}_i$ , the active force on each bead  $i$  is modeled as:

$$\mathbf{f}_i^a = \frac{f^a}{\ell}(\mathbf{r}_{i,i+1} + \mathbf{r}_{i-1,i}), \quad (4)$$

which mimics a homogeneous active force driving along the backbone of the chain. Here,  $f^a$  is the strength of active force,  $\ell$  is the mean bond length and the orientation of force on end beads is parallel to end bonds. The thermal noise  $\mathbf{f}_i^r$  in Eq. (1) is a delta correlated random force acting on particle  $i$  with zero mean and strength  $2D_0\gamma^2$

$$\langle \mathbf{f}_i^r(t) \mathbf{f}_j^r(t') \rangle = 2D_0\gamma^2 \delta_{ij} \delta(t - t'), \quad (5)$$

where  $D_0$  is the diffusion coefficient of a single passive monomer particle, the  $\delta_{ij}$  is the Kronecker delta and  $\delta(t - t')$  is the Dirac delta.

In the overdamped limit, where we can neglect inertial effects, the Langevin equations of motion Eq.(1) result in Brownian Dynamics equations of motion:

$$\gamma\dot{\mathbf{r}}_i = - \sum_j \nabla_{\mathbf{r}_i} U(r_{ij}) + \mathbf{f}_i^a + \mathbf{f}_i^r \quad (6)$$

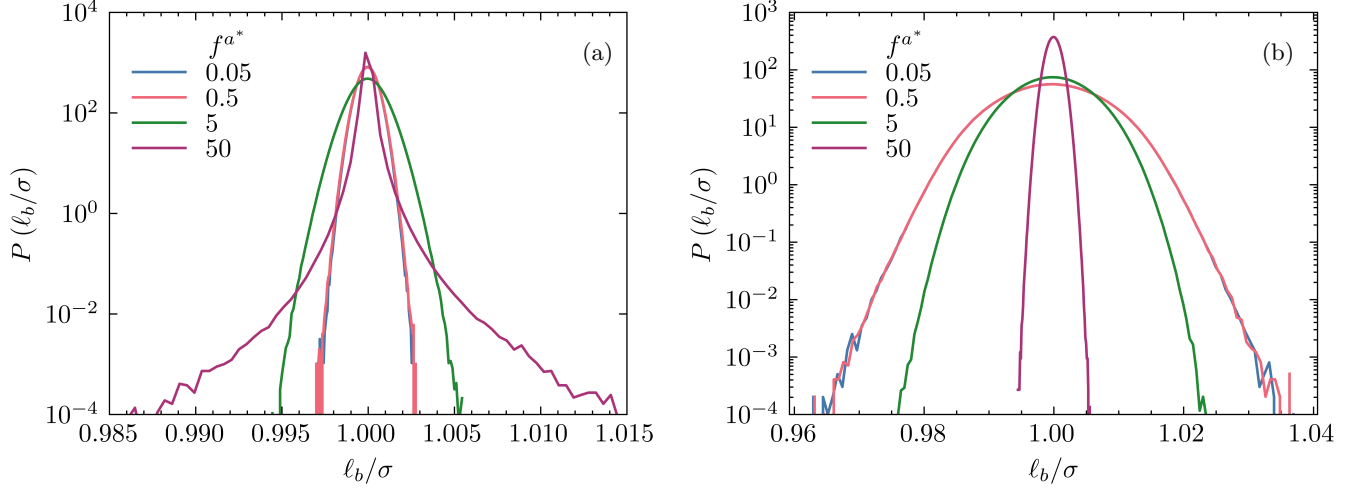

FIG. S1. a) PDF of bond length for underdamped chains of  $N = 500$  and different activities. b) Same graph for overdamped polymers.

| $N$ | $f^{a*}$ | $N_{run}$ | $N_{pro}$ | $dt$    | $k_s^*$ |
|-----|----------|-----------|-----------|---------|---------|
| 500 | 0.01     | 5.0e+08   | 9.0e+08   | 1.0e-03 | 1.0e+06 |
| 500 | 0.025    | 3.6e+08   | 3.6e+08   | 1.0e-03 | 1.0e+06 |
| 500 | 0.05     | 1.8e+08   | 1.8e+08   | 1.0e-03 | 1.0e+06 |
| 500 | 0.1      | 9.0e+07   | 9.0e+07   | 1.0e-03 | 1.0e+06 |
| 500 | 0.25     | 3.6e+07   | 3.6e+07   | 1.0e-03 | 1.0e+06 |
| 500 | 0.5      | 1.8e+07   | 1.8e+07   | 1.0e-03 | 1.0e+06 |
| 500 | 1        | 9.0e+06   | 9.0e+06   | 1.0e-03 | 1.0e+06 |
| 500 | 2.5      | 9.0e+06   | 9.0e+06   | 1.0e-03 | 1.0e+06 |
| 500 | 5        | 9.0e+06   | 9.0e+06   | 1.0e-03 | 1.0e+06 |
| 500 | 10       | 9.0e+06   | 9.0e+06   | 1.0e-03 | 1.0e+06 |
| 500 | 25       | 1.8e+07   | 1.8e+07   | 2.0e-04 | 1.0e+07 |
| 500 | 50       | 1.8e+07   | 1.8e+07   | 1.0e-04 | 1.0e+07 |
| 500 | 100      | 4.0e+07   | 4.0e+07   | 5.0e-05 | 1.0e+07 |

| $N$ | $f^{a*}$ | $N_{run}$ | $N_{pro}$ | $dt$    | $k_s^*$ |
|-----|----------|-----------|-----------|---------|---------|
| 500 | 0.01     | 6.8e+08   | 6.8e+08   | 1.0e-04 | 5.0e+03 |
| 500 | 0.025    | 9.0e+08   | 9.0e+08   | 1.0e-04 | 5.0e+03 |
| 500 | 0.05     | 9.0e+08   | 9.0e+08   | 1.0e-04 | 5.0e+03 |
| 500 | 0.1      | 9.0e+08   | 9.0e+08   | 1.0e-04 | 5.0e+03 |
| 500 | 0.25     | 3.6e+08   | 3.6e+08   | 1.0e-04 | 5.0e+03 |
| 500 | 0.5      | 1.8e+08   | 1.8e+08   | 1.0e-04 | 5.0e+03 |
| 500 | 1        | 1.8e+08   | 1.8e+08   | 1.0e-04 | 5.0e+03 |
| 500 | 2.5      | 9.0e+07   | 9.0e+07   | 5.0e-05 | 5.0e+03 |
| 500 | 5        | 1.8e+08   | 1.8e+08   | 5.0e-05 | 5.0e+03 |
| 500 | 10       | 9.0e+07   | 9.0e+07   | 1.0e-05 | 5.0e+03 |
| 500 | 25       | 9.0e+07   | 9.0e+07   | 1.0e-06 | 1.0e+05 |
| 500 | 50       | 9.0e+07   | 9.0e+07   | 1.0e-06 | 1.0e+05 |
| 500 | 100      | 4.5e+07   | 4.5e+07   | 1.0e-06 | 1.0e+05 |

TABLE I. Summary of simulation for  $N = 500$  for underdamped (left) and overdamped (right) cases. The tables contains the information about the number of thermalizing steps  $N_{run}$  before the actual simulation and then the total production steps of  $N_{pro}$ , the corresponding step size  $dt$  and the bond spring constants for each activity.

## B. Dimensionless groups and simulation details

The simulations are carried out in HOOMD-BLUE [2] package with home-made modification to include the active force using a GPU implementation. The equations of motion are solved using a velocity-Verlet scheme.

We choose  $\ell_u = \sigma$ ,  $E_u = \epsilon$  and  $\tau_u = \gamma\sigma^2/\epsilon$ , with  $\gamma = 1$ , as the units of length, energy and time, respectively and reduced quantities are denoted by  $*$  superscript. We fix  $\ell/\sigma = 1$  and dimensionless diffusion coefficient  $D_0^* = 0.1$ , whereas we vary dimensionless active force strength  $f^{a*} = \frac{f^a\sigma}{\epsilon}$  in the range  $0.01 \leq f^{a*} \leq 100$  for chain lengths  $50 \leq N \leq 1000$ . The reduced mass  $m^* = m\epsilon/(\gamma\sigma)^2 = 1$  is varied in the range  $0 \leq m^* \leq 5$ . However, the majority of simulations focus on the overdamped limit  $m^* = 0$  and the underdamped case of  $m^* = 1$ . The spring constant of bond potential  $k_s^* = k_s\sigma^2/\epsilon$  is chosen according to active force strength, such that the maximum bond length fluctuation is less than 5% of average bond length which is  $\sigma$ , see Table I for the chosen values of  $k_s^*$ . Fig. S1 shows the distribution of bond length in simulations, which is defined as  $\ell_b = |\mathbf{r}_{i+1}(t) - \mathbf{r}_i(t)|$  for  $i$ th monomer, at several  $f^{a*}$ .

To produce the desired statistics, for each set of parameters *i.e.*,  $(N, f^{a*})$  we have simulated 120 independent chain configurations. For this purpose, we first equilibrated passive polymers of different chain lengths and then we used them as starting configurations for active polymers. The simulations consist of  $N_{run}$  timesteps until the polymers reach a dynamical steady state, to ensure that no vestige of the initial conditions are remained. Subsequently they are followed by a production run of  $N_{pro}$  timesteps to compute the structural and dynamical observable quantities.

We verified that the total time in the production run  $t_{pro} = n_{pro} * dt$  is at least four times larger than the relaxation time of the end-to-end vector  $\tau_e^*$ . A summary of simulation parameters, including timestep  $dt$  can be found in Table I.

## II. CONFORMATIONAL PROPERTIES

The asphericity  $A$  of polymers is defined as [3]

$$A = \frac{\langle Tr^2 - 3M \rangle}{\langle Tr^2 \rangle}, \quad (7)$$

where  $Tr = \lambda_1 + \lambda_2 + \lambda_3$ ,  $M = \lambda_1\lambda_2 + \lambda_2\lambda_3 + \lambda_3\lambda_1$  and each  $\lambda$  is an eigenvalue of the  $3 \times 3$  gyration tensor. It ranges from 0 for perfect spherical conformation to 1 for rod-like one. Fig. S2 shows the asphericity  $A$  of active polymers against  $f^{a^*}$  for chains in the underdamped and overdamped regimes. While  $A$  of inertial chains exhibits a striking increase for  $f^{a^*} > 1$  indicating an elongated shape, the asphericity of overdamped chains decreases slightly with  $f^{a^*}$ , akin to the trends observed in reference [4] for a similar model.

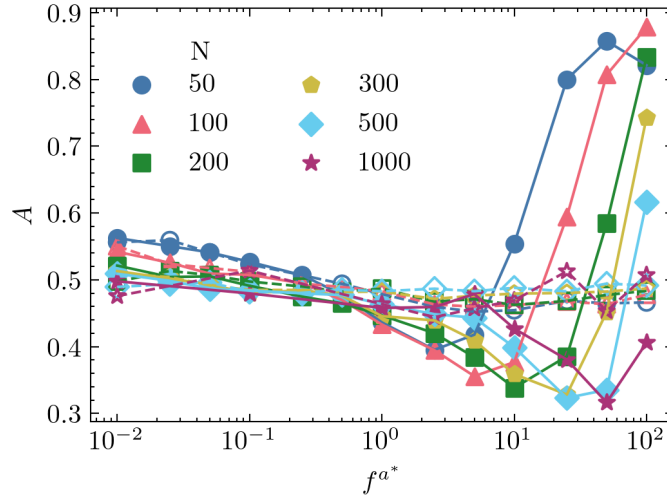

FIG. S2. Asphericity  $A$  of active polymers of different chain lengths  $50 \leq N \leq 1000$  as a function of  $f^{a^*}$  in the underdamped (bold symbols) and overdamped (empty symbols) regimes.

The probability distribution function (PDF) of end-to-end distance  $R_e^*$  is shown in Fig. S3. More extended shape of active inertial chains at high activities can be inferred from a broader distribution of their  $P(R_e^*)$ . For overdamped active chains, we observed a slightly more peaked  $P(R_e^*)$  at high activities, reflecting their conformational shrinkage, similar to reference [4].

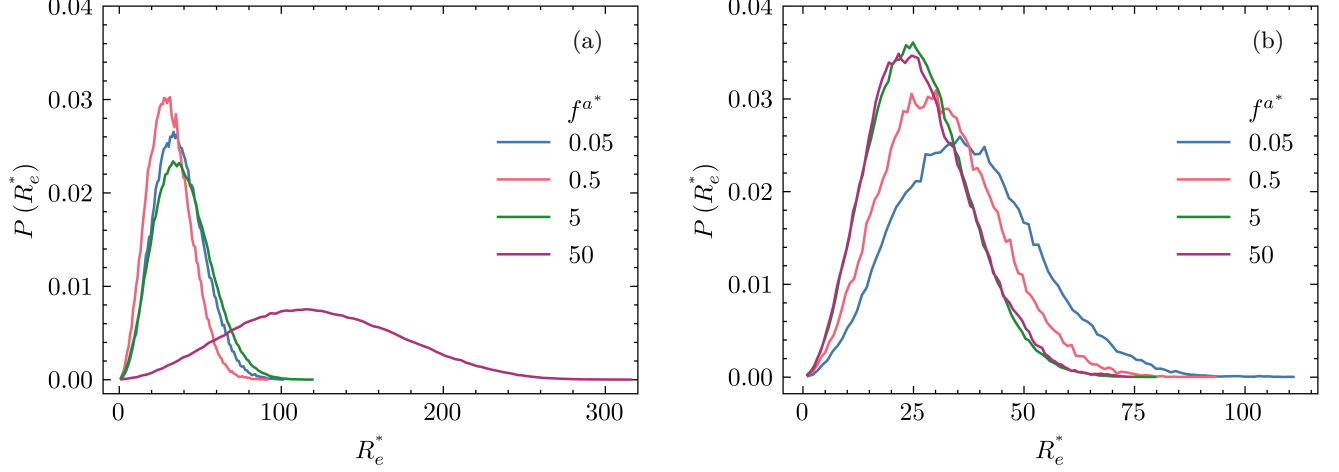

FIG. S3. PDF of end-to-end distance for active chains of  $N = 500$  at different activities with (a) underdamped and (b) overdamped dynamics.

As stated in the main article, we assumed a scaling form  $\langle R_e^{*2} \rangle = C_\infty(f^{a*})N^{2\nu(f^{a*})}$  for end-to-end distance. To demonstrate the validity of our scaling ansatz, in Fig. S4 we have plotted  $R_e^{*2}$  of all active inertial polymers for different  $N$  and  $f^{a*}$  normalised to their corresponding  $C_\infty$  versus  $N^{\nu(f^{a*})}$ . All the data collapse on a line, verifying the validity of our scaling hypothesis.

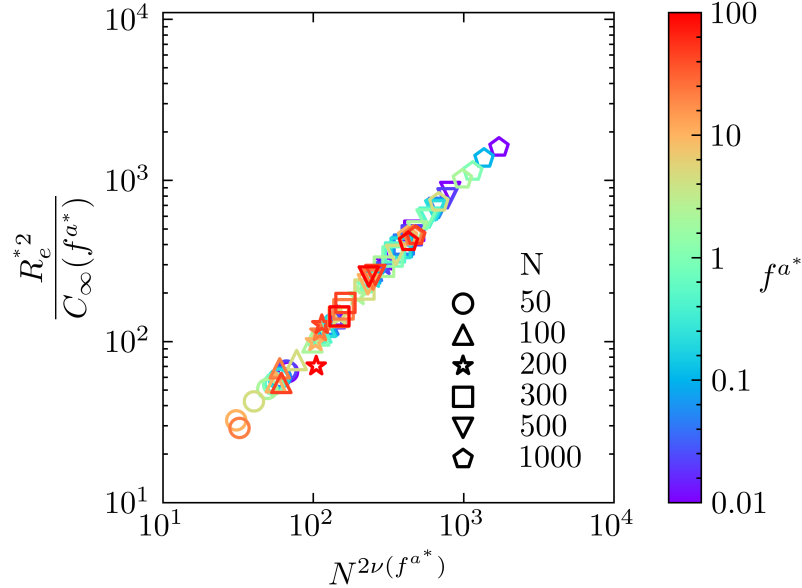

FIG. S4. The normalised  $\frac{R_e^{*2}}{\ell_b^2 C_\infty(f^{a*})^2}$  as a function of  $N^{2\nu(f^{a*})}$  for underdamped chains. N.B, we excluded the outliers of  $R_e^*$ , which are  $(N, f^{a*}) \in \{(50, 50), (50, 100), (100, 100)\}$ .

To obtain the persistence length, we compute the orientational bond-bond correlation function  $\langle \cos \theta(s) \rangle$  defined as the cosine of the angle between any two bonds whose curvilinear distance is  $s$ . Figs. S5 (a) and S5(b) present the  $\langle \cos \theta(s) \rangle$  at different activities for inertial and overdamped chains, respectively. For both cases, the bond-bond correlation function develops a negative dip at intermediate  $s$ , indicating a local back-folding of active chains. For inertial chains, the bond orientational correlation along backbone becomes larger upon increase of activity and the negative dip appears at larger  $s$ , whereas for overdamped active chains the decay length is weakly affected by

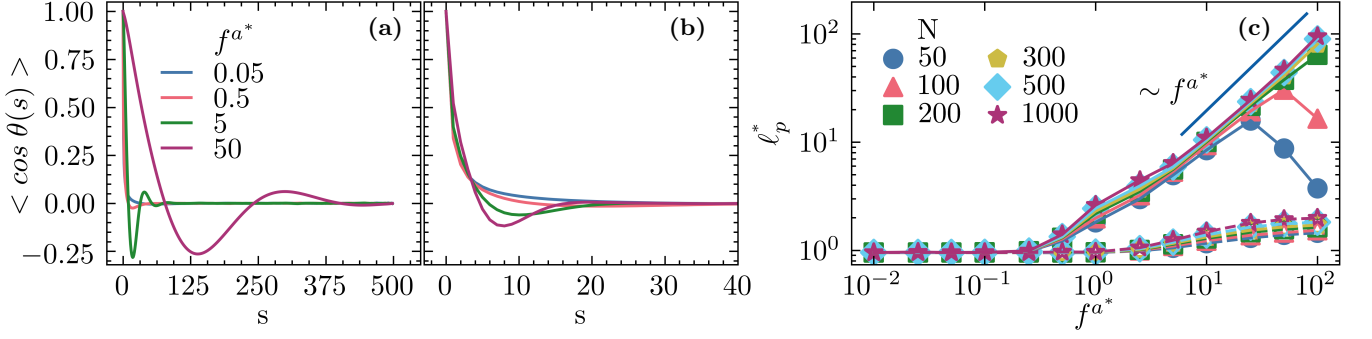

FIG. S5. (a) and (b) Bond-bond orientational correlation function against curvilinear distance  $s$  for inertial and overdamped chains with  $N = 500$  at different activities, respectively. (c) Dependence of persistence length  $\ell_p^*$  on  $f^{a*}$  for inertial (bold symbols) and overdamped (empty symbols) polymers of different lengths.

activity. As  $\langle \cos \theta(s) \rangle$  does not decay exponentially, we define persistence length  $\ell_p^*$  as the curvilinear distance at which  $\langle \cos \theta(\ell_p^*) \rangle = 1/e$ .

### III. VIDEOS

Videos of the time evolution of an active polymer configuration starting from a passive state have been provided. These include one video for an overdamped active chain and two videos for an inertial active polymer. In all of them, the chain length is  $N = 500$  and  $f^{a*} = 100$ . To show the polarity of polymer, the four starting monomers are colored in blue and the rest of monomers are red. The specification of the videos are as follows:

The video file "LD-N500-f100.mp4" is for inertial polymer including the period that it reaches a steady state. The video file "LD-N500-f100-zoomed.mp4" also shows the same active inertial chain, however with a more zoomed-up view for a more detailed visualisation of the transition from coil-like to elongated configuration in the steady-state due to impacts from inertial collisions. The snapshots are recorded each 2000 timesteps with  $dt = 5 \times 10^{-5}$ .

Finally, the video file "BD-N500-f100.mp4" is for overdamped polymer and shows how the chain tends to swirl around itself like a yarn ball. The snapshots are recorded each 20000 timesteps with  $dt = 10^{-6}$ .

#### A. Mass dependence of mean conformational properties

We have studied the dependence of end-to-end distance and persistence length on mass while keeping all other parameter constant. Fig. S6(a) and S6(b) show end-to-end distance and persistence length for active polymer of chain length  $N = 500$  with reduced active force  $f^{a*} = 10$ . We see that both quantities systematically increase with  $m^*$  and specially for  $\tau_m^*/\tau_{adv}^* > 1$  both the  $R_e^*$  and  $\ell_p^*$  are almost linear in mass  $m^*$ .

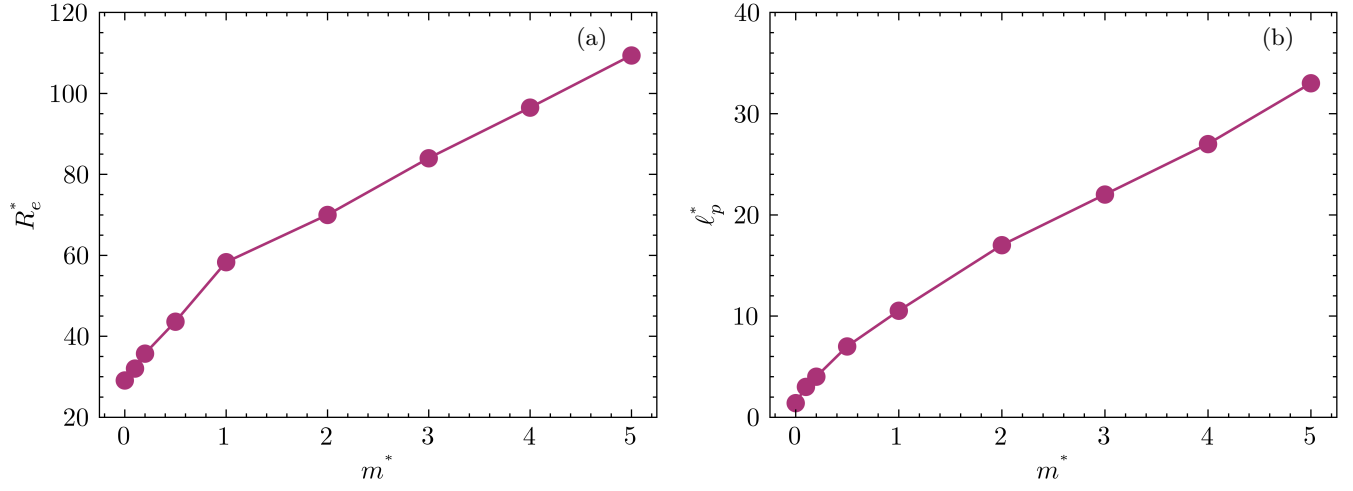

FIG. S6. a) Dependence of  $R_e^*$  on the reduced mass  $m^*$  for chain length of  $N = 500$  and activity of  $f^{a^*} = 10$ . b) Dependence of  $\ell_p^*$  on mass for chain length of  $N = 500$  and activity of  $f^{a^*} = 10$ .

#### IV. DYNAMICAL PROPERTIES

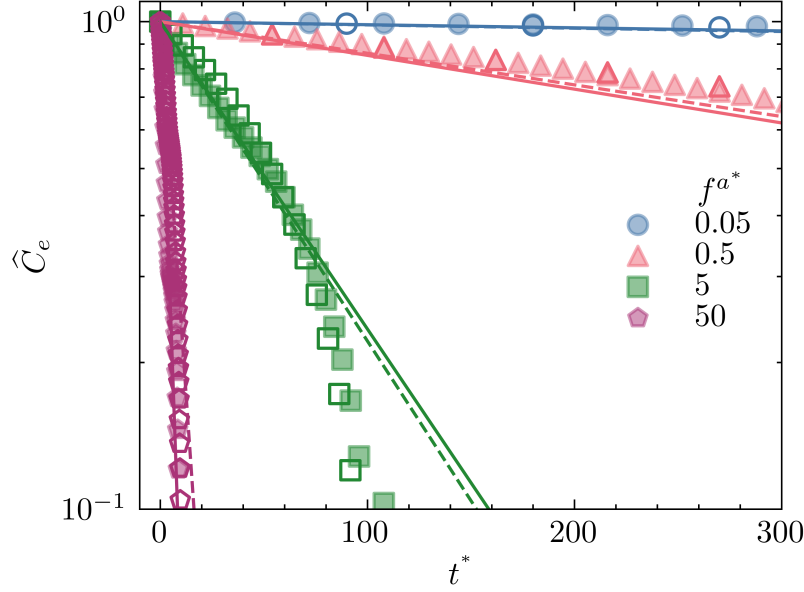

FIG. S7. Normalized end-to-end vector TACF for chains of  $N = 500$  and different activities (symbols) and their corresponding exponential fits (lines)  $\hat{C}_e = \exp(-t^*/\tau_e^*)$ . The bold symbols and solid lines correspond to inertial active chains, whereas empty symbols and dashed lines represent the overdamped active chains.

##### A. Exponential decay of $C_e^*$

In Fig. S7,  $\hat{C}_e = \lim_{t' \rightarrow \infty} \langle \mathbf{R}_e(t+t') \cdot \mathbf{R}_e(t') \rangle / \langle \mathbf{R}_e^2(t') \rangle$  is fitted by exponential functions with the form  $\exp(-t^*/\tau_e^*)$  and the  $\tau_e^*$  for each  $N$  correspond to the times that their normalized end-to-end vector time correlation function  $\hat{C}_e$  reaches the value of  $1/e$ .

##### B. Mean-squared displacement of center of mass

In Fig. S8, the mean squared displacement of the center of mass is shown. We extract the long-time diffusion coefficient, from the slope of MSD at times  $t^* > \tau_e^*$ , where it grows linearly with time  $t^*$ . The difference in center of mass dynamics between underdamped and overdamped chains regarding their initial behavior is visible at

for larger activities, when  $f^* \geq 5$ . For less active chains there exists an initial short time diffusive regime as well as the long time one. Despite that all the chains are in their steady state hence they have a center of mass velocity when we begin to capture their dynamics, at the beginning, in contrast to highly activated chains, the passive diffusion by the thermal forces wins over activity for less active polymers. Therefore, we see an initial diffusion followed by an active ballistic regime which finally reaches another diffusive behaviour for these chains.

##### C. Velocity correlations

We compute time autocorrelation function of the center of mass velocity normalized by the long-time mean-squared velocity of center of mass in the steady-state limit  $\hat{C}_v(t) = \lim_{t' \rightarrow \infty} \langle \mathbf{V}_{cm}(t+t') \cdot \mathbf{V}_{cm}(t') \rangle / \langle \mathbf{V}_{cm}^2(t') \rangle$ , where  $\mathbf{V}_{cm}(t) = \frac{1}{N} \sum_{i=1}^N \mathbf{v}_i$ . Fig. S9 (a) and (b) show  $\hat{C}_v$  for underdamped and overdamped active polymers of  $N = 500$  at different  $f^{a*}$ , respectively. Unlike passive systems, we observe a finite relaxation of  $\hat{C}_v$  even for the overdamped dynamics. For the underdamped active chains, we recognize an initial fast decay around  $\tau_m^* = 1$  in addition to a longer decay time which is similar to that of the overdamped chains. For both kinds of dynamics, the characteristic relaxation

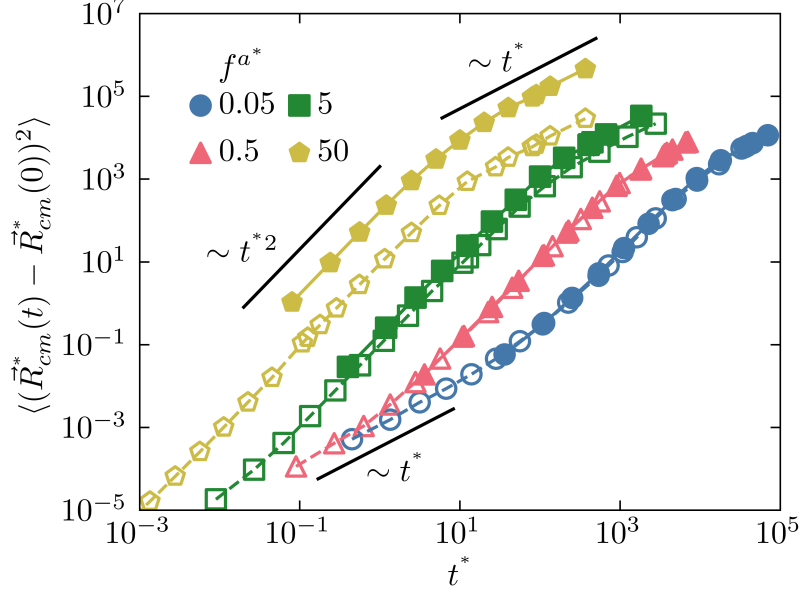

FIG. S8. Mean squared displacement of center of mass for chains of  $N = 500$  and different activities for underdamped (filled) and overdamped (empty) polymers.

times of  $\hat{C}_v$  decrease with  $f^{a^*}$ , similar to trends observed for  $\hat{C}_e$ . In Figs. S9 (c) and (d), we have presented  $\langle \mathbf{V}_{cm}^{*2} \rangle$  as a function of  $f^{a^*}$  for underdamped and overdamped dynamics. For inertial chains, the mean-squared velocity is almost independent of  $f^{a^*}$  for  $f^{a^*} < 1$ , whereas for large active forces it grows steeper than  $f^{a^*2}$ . In the overdamped dynamics, we observe a weak decrease of  $\langle \mathbf{V}_{cm}^{*2} \rangle$  for small  $f^{a^*}$  but it grows as  $f^{a^*2}$  for larger activities. Nevertheless, the mean-squared velocities of inertial chains at large activities are one order of magnitude larger.

## V. ANALYTICAL CALCULATIONS OF CENTER OF MASS DYNAMICS

The dynamics of center of mass velocity is obtained by summing the equations of motions of all the beads given by Eq. (1). As contributions from the internal forces cancel out, the equation for  $\mathbf{V}_{cm}(t)$  simplifies to:

$$m\dot{\mathbf{V}}_{cm} = -\gamma\mathbf{V}_{cm} + \frac{1}{N}(\mathbf{F}^a + \mathbf{F}^r) \quad (8)$$

in which  $\mathbf{F}^r = \sum_{i=1}^N \mathbf{f}_i^r$  is a sum of all the random forces with a zero mean and  $\langle \mathbf{F}^r(t) \cdot \mathbf{F}^r(t') \rangle = 6ND_0\gamma^2\delta(t - t')$ . Integrating this first-order differential equation yields

$$\begin{aligned} \mathbf{V}_{cm}(t) = & \mathbf{V}(t_0)e^{-\frac{\gamma}{m}(t-t_0)} \\ & + \frac{1}{Nm} \int_{t_0}^t d\tau [\mathbf{F}^a(\tau) + \mathbf{F}^r(\tau)] e^{-\frac{\gamma}{m}(t-t_0-\tau)} \end{aligned} \quad (9)$$

Using this solution, we calculate the velocity TACF in the steady-state limit:

$$\begin{aligned} C_v(t) = & \frac{3\gamma D_0}{Nm} e^{-\frac{t}{\tau_m}} \\ & + \frac{1}{2m\gamma N^2} \int_0^{+\infty} \left[ C_f(u-t) + C_f(u+t) \right] e^{-\frac{u}{\tau_m}} du., \end{aligned} \quad (10)$$

in which  $C_f(t) = \lim_{t' \rightarrow \infty} \langle \mathbf{F}^a(t+t') \cdot \mathbf{F}^a(t') \rangle$  is the TACF of the total active force. The first term in Eq. (10) represents the passive diffusive contribution from random forces which decays exponentially with relaxation time  $\tau_m$  [5], whereas the second term entangles the correlation of the total active force with inertial relaxation. This term reflects memory effects induced by active forces and accounts for the emergent inertial effects. In the limit of vanishing mass,  $C_v$  simplifies to

$$\lim_{m \rightarrow 0} C_v(t > 0) = \left(\frac{1}{N\gamma}\right)^2 C_f(t). \quad (11)$$

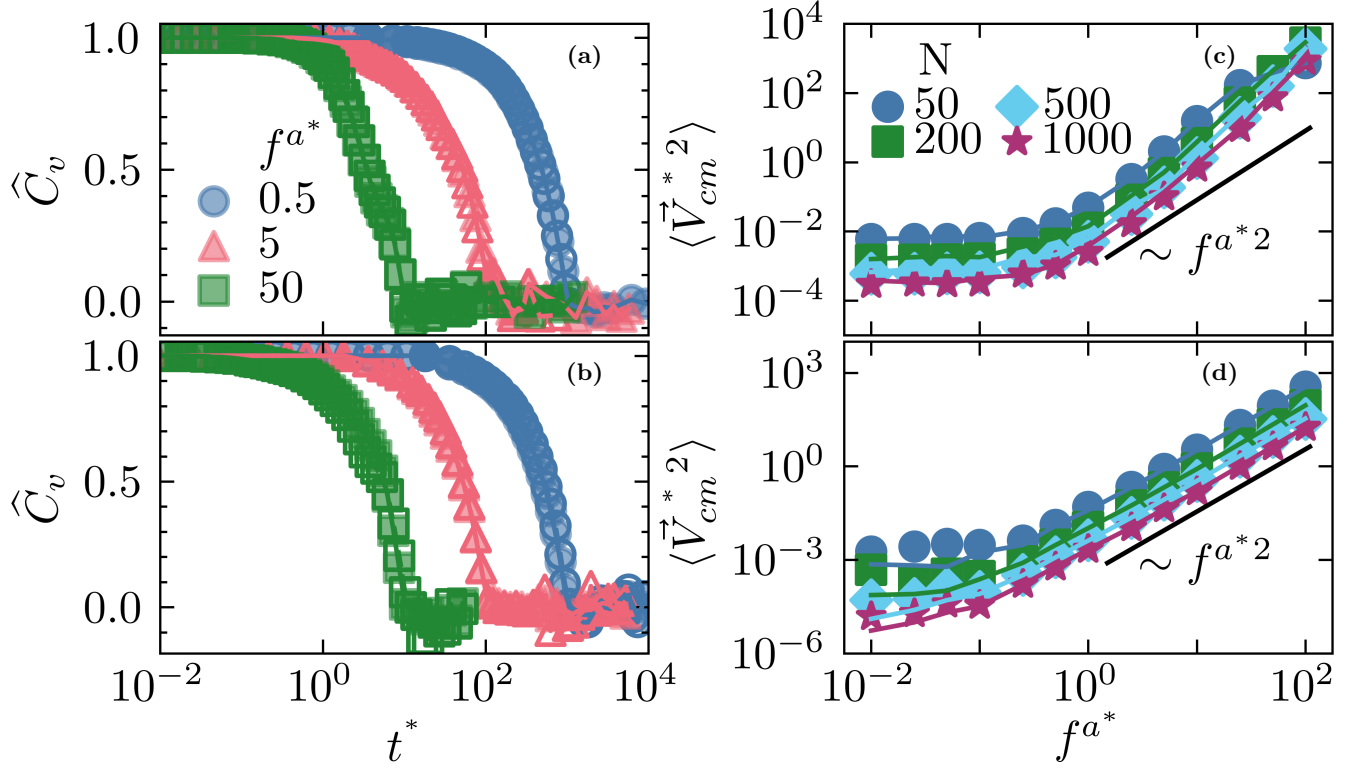

FIG. S9. (a) and (b) Normalized Center of mass velocity TACF for active polymers of  $N = 500$  and different activities, in the underdamped and overdamped regimes, respectively. The bold symbols are obtained directly from simulations, whereas empty ones show predictions of Eq. (10) and Eq. (11) using  $C_e$  from simulations. (c) and (d) The mean-squared velocity of center of mass versus  $f^a$  for different chain lengths, color codes are given in the legends, in the underdamped and overdamped regimes, respectively. The lines show theoretical predictions of Eq. (12) and Eq. (13).

Predictions of Eq. (10) and Eq. (11) using  $\langle R_e^2 \rangle$  and  $\hat{C}_e(t)$  from simulations as an input are included in Figs. S9 (a) and (b), showing excellent agreement with simulation results.

Next, we obtain the steady-state mean-squared center of mass velocity for tangentially-driven polymers from Eq. (10), yielding

$$\lim_{t \rightarrow \infty} \langle \mathbf{V}_{cm}^2(t) \rangle = \frac{3\gamma D_0}{Nm} + \frac{f^a}{m\gamma N^2} \frac{\langle R_e^2 \rangle}{\ell^2} \int_0^{+\infty} \hat{C}_e(u) e^{\frac{-u}{\tau_m}} du. \quad (12)$$

The mean-squared velocity for small  $f^a$  is dominated by the diffusive term, whereas for  $\frac{f^a}{3N\gamma^2 D_0} \frac{\langle R_e^2 \rangle}{\ell^2} > 1$ , it is determined by the active contribution. For sufficiently large  $f^a$  such that the relaxation time  $\tau_e < \tau_m$ ,  $\int_0^{+\infty} \hat{C}_e(u) e^{\frac{-u}{\tau_m}} du \approx \tau_e$ . In this limit,  $\langle \mathbf{V}_{cm}^2 \rangle(f^a \gg 1) = \frac{f^a}{m\gamma N^2} \frac{\langle R_e^2 \rangle}{\ell^2} \tau_e$ . Using  $\tau_e = AN/f^a$  and the scaling behavior of  $\langle R_e^2 \rangle$  it becomes proportional to  $f^{a2} N^{2\nu(f^a)-1}$ . Eq. 12 in the limit of vanishing mass simplifies to

$$\lim_{m \rightarrow 0} \langle \mathbf{V}_{cm}^2(t \gg 1) \rangle = \frac{f^{a2} \langle R_e^2 \rangle}{(\ell^2 N \gamma)^2}. \quad (13)$$

Predictions of Eq.(12) and Eq. (13) compared with  $\langle \mathbf{V}_{cm}^2(0) \rangle$  computed in simulations are presented in Fig. S9 (c) and (d) showing very good agreement.

## VI. THE ACTIVE BROWNIAN POLYMER

The very basic model for active chains is a sequence of active Brownian particles connected with springs, forming an Active Brownian Polymer (ABPO).

A flexible ABPO is composed of  $N$  active Brownian particles ( $i = 1, \dots, N$ ), which their dynamics is described by the following equation of motion:

$$m\ddot{\mathbf{r}}_i(t) = -\gamma_T \dot{\mathbf{r}}_i(t) + \gamma_T v_0 \mathbf{e}_i(t) - \sum_j \nabla_{\mathbf{r}_i} U(r_{ij}) + \mathbf{f}_i^r(t) \quad (14)$$

$$\dot{\mathbf{e}}_i(t) = \hat{\boldsymbol{\eta}}_i(t) \times \mathbf{e}_i(t) \quad (15)$$

Where  $\mathbf{r}_i$  is the position of particle  $i$ , and  $\gamma_T v_0 \mathbf{e}_i(t)$  is the active self-propulsion with the speed of  $v_0$  and direction of  $\mathbf{e}_i(t)$  which diffuses according to eqn (15).  $\gamma_T$  is the translational friction and the forces between all other particle  $j$  and particle  $i$  is given by the the same two potentials  $U_{r_{ij}} = U_{\text{Harmonic}} + U_{\text{excl.}}$ .

The noise terms  $\mathbf{f}_i^r$  and  $\boldsymbol{\eta}_i$  are Gaussian and Markovian stochastic processes with mean value of zero and second moments of:

$$\langle \mathbf{f}_i^r(t) \cdot \mathbf{f}_j^r(t') \rangle = 6D_0 \gamma^2 \delta_{ij} \delta(t - t') \quad (16)$$

$$\langle \boldsymbol{\eta}_i(t) \boldsymbol{\eta}_j(t') \rangle = 2D_r \delta_{ij} \delta(t - t') \quad (17)$$

in which,  $D_0$  is the single passive particle diffusion coefficient and  $D_r$  is the rotational diffusion coefficient. The correlation of the orientation vector  $\mathbf{e}_i$  is given by [6]

$$\langle \mathbf{e}_i(t) \cdot \mathbf{e}_i(t') \rangle = e^{-2D_r |t - t'|}, \quad (18)$$

where  $\tau_r = 1/(2D_r)$  denotes the rotational relaxation time.

Noting that the total active force on an ABPO of chain length  $N$  is  $\mathbf{F}^a = \gamma^T v_0 \sum_{i=1}^N \mathbf{e}_i$ , its time autocorrelation function using eq. (18) becomes

$$C_f = \langle \mathbf{F}^a(0) \cdot \mathbf{F}^a(t) \rangle = N(\gamma^T v_0)^2 e^{-|t|/\tau_r}, \quad (19)$$

For inertial chains of this type (ABPO), velocity auto-correlation can be obtained from Eq. (10) using the explicit form of active force auto-correlation given by Eq. (19).

$$C_v^{ABPO}(s) = \frac{3D_0\gamma_T}{Nm} e^{\frac{-s}{\tau_m}} + \frac{v_0^2}{N} \frac{\tau_r}{\tau_r^2 - \tau_m^2} \left[ \tau_r e^{-s/\tau_r} - \tau_m e^{-s/\tau_m} \right]. \quad (20)$$

We can also find the long time diffusion coefficient as follows,

$$D_L = \frac{1}{3} \int_0^\infty C_v(t) dt = \frac{D_0}{N} + \frac{v_0^2 \tau_r}{3N}, \quad (21)$$

which turns out to be independent of  $\tau_m$ , similar to the case of inertial ABPs without orientational inertia [6]. For non-inertial ABPOs we have,

$$\lim_{m \rightarrow 0} C_v(s > 0) = \frac{v_0^2}{N} e^{-|t|/\tau_r}, \quad (22)$$

$$\lim_{m \rightarrow 0} D_L = \frac{D_0}{N} + \frac{v_0^2 \tau_r}{3N}. \quad (23)$$

On panel (a) of Fig.S10 we see the predictions of eq. (20) and eq. (22) show very good agreement with the results of simulations for the velocity auto-correlation of ABPOs and the differences between inertial and overdamped cases. We normalised all the values with respect to the squared center of mass velocities that are predicted by theory, which gives  $\langle \mathbf{V}_{cm}^{*2} \rangle = 0.71$  for the ABPO with inertia and  $\langle \mathbf{V}_{cm}^{*2} \rangle = 5$  for the overdamped one for this particular chain length and active force strength. Furthermore, using eq. 21 and eq. 23 for long time diffusion coefficients of ABPOs, we have  $D_L/D_0 = 2.77$  for both inertial and overdamped cases (N.B, the two formulas are identical and mass-independent). From the simulations, we have found that for inertial case  $D_L/D_0 = 2.62$  and for overdamped one  $D_L/D_0 = 2.59$ .

Finally, we report the end-to-end distance of each case. For inertial ABPO it is  $R_e^* = 57.4$  and for overdamped one we have  $R_e^* = 53.4$ , which seems that the two cases are having quite the same size. This shows the impact of inertia on the size of active chains are much more significant when the active driving force is tangential.

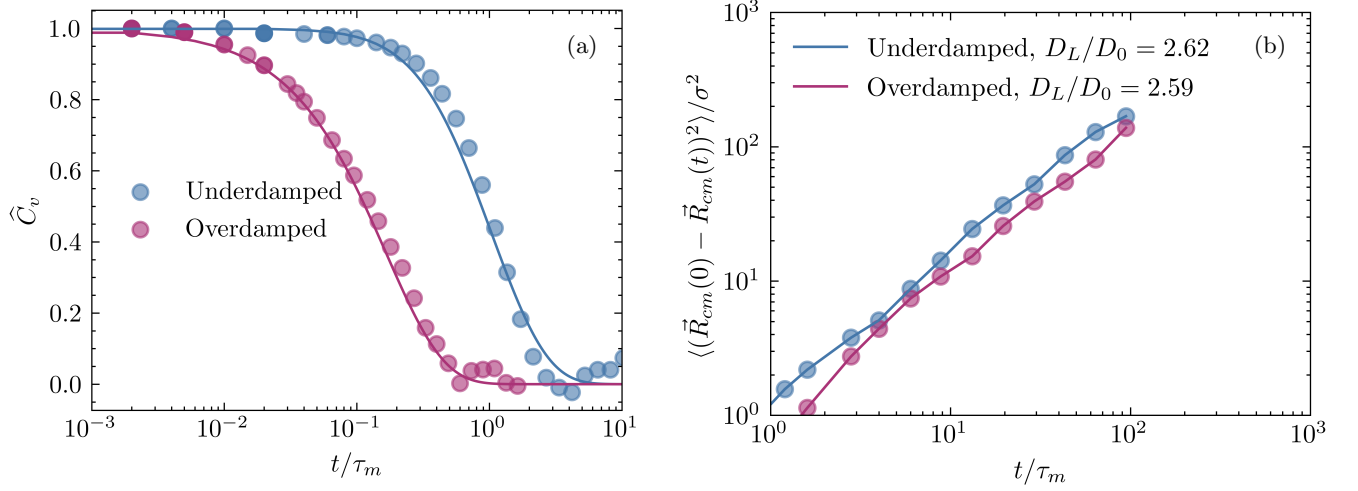

FIG. S10. a) Comparison of the normalised velocity auto-correlation functions of underdamped (inertial) and overdamped ABPOs with their corresponding analytical predictions, namely eq. (20) and eq. (22) which are plotted in solid blue and purple lines respectively. The chains are both active with  $v_0^* = 50$  (in the same dimension-less system as tangentially driven ones) and chain length of  $N = 500$ . b) Comparison of the MSDs of the overdamped and underdamped ABPOs. **show the MSDs by symbols.**

- 
- [1] R. E. Isele-Holder, J. Elgeti, and G. Gompper, *Soft Matter* **11**, 7181 (2015).
  - [2] J. A. Anderson, J. Glaser, and S. C. Glotzer, *Computational Materials Science* **173**, 109363 (2020).
  - [3] J. Rudnick and G. Gaspari, *Journal of Physics A: Mathematical and General* **19**, L191 (1986).
  - [4] V. Bianco, E. Locatelli, and P. Malgaretti, *Phys. Rev. Lett.* **121**, 217802 (2018).
  - [5] C. P. J. Wong and P. Choi, *Computational Materials Science* **155**, 320 (2018).
  - [6] H. Lowen, *The Journal of Chemical Physics* **152**, 040901 (2020).
